# Supplementary material for: A Novel Electrochemical Flow-Cell for Operando XAS Investigations On X-ray Opaque Supports
Source: arXiv:2309.16184 source file (2023-09-28)
Supplement: Supplementary file 1 [file Supporting_Info.pdf]

# A NOVEL ELECTROCHEMICAL FLOW-CELL FOR *OPERANDO* XAS INVESTIGATIONS ON X-RAY OPAQUE SUPPORTS – SUPPORTING INFORMATION.

F. Paparoni,[1, 2] G. Alizon,[2] A. Zitolo,[2] A. Di Cicco,[1] S. J. Rezvani[1,4], H. Magnan,[3] and E. Fonda[2]

[1]Sez. Fisica, Scuola di Scienze e Tecnologie, Università di Camerino, via Madonna delle Carceri, I-62032 Camerino, Italy.
[2]Synchrotron SOLEIL, L'Orme des Merisiers, BP48 Saint Aubin, 91192 Gif-sur-Yvette, France.
[3]Université Paris-Saclay, CEA, CNRS, Service de Physique de l'Etat Condensé, F-91191 Gif-sur-Yvette, France.
[4]CNR-IOM, SS14 – km 163.5 in Area Science Park, 34149, Trieste, Italy.

## S1. DETERMINATION OF NI CONTENT

Samples were probed with XPS. All Fe 2p spectra (Fig. 1S-a) confirm the formation of $Fe_2O_3$, with a main Fe $2p_{3/2}$ line at 710.9 eV and shakeup satellite at 718.7 eV in agreement with the presence of the $Fe^{3+}$ oxidation state [1]. The Ni 2p spectra (Fig. 1S-b) highlight the higher Ni content within sample pt45 with respect to pt43, as proven by increasing Ni 2p intensities, and similarity with the spectra to a $NiFe_2O_4$ reference [2]. The position of the Ni $2p_{1/2}$ and Ni $2p_{3/2}$ lines are in agreement with the presence of $Ni^{2+}$. Ni/Fe ratios were determined from XPS data using the CASAXPS software [15].

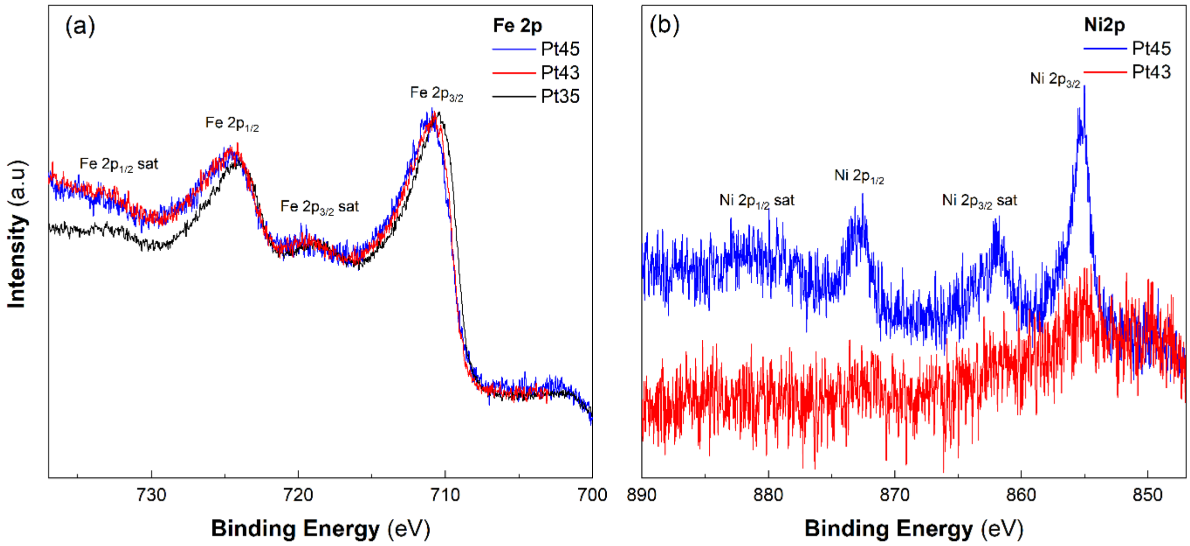


***Figure 1S.*** XPS spectra of the Ni-doped maghemite samples: (a) Fe 2p, (b) Ni 2p.

However, as shown by figure 1S-b, the very low intensity of the Ni 2p for sample pt43, due to the very low Ni content, lead to a high relative error associated to the calculation. To have a better determination of the Ni/Fe ratios, samples were investigated via X-ray fluorescence spectroscopy (XRF). Using the bending-magnet radiation of the SAMBA beamline, XRF spectra were acquired from the samples using a beam energy ($E_b$) of 8600 eV. Five scans were collected for each sample. XRF analysis highlight the presence of Iron, Nichel and a very small signal coming from the M emission line of the Pt substrate (see Fig. S2). The argon peaks can be expected when performing a fluorescence experiment in air. Quantitative XRF analysis was carried out by fitting the $K_\alpha$ emission lines of Fe and Ni, after the background removal. The value of the maximum intensity of the two function ($I_{Fe}$ and $I_{Ni}$) was extracted for each scan and the obtained values were averaged. The error was estimated equal to the higher standard deviation between the measurements. The calculation was carried out following the procedures discussed in the doctoral thesis of McBriarty [3] and Klung [4]. In this case, considering that the dead time correction for the Si detector is applied by the acquisition software and that the detector efficiency is ~1 at both energies, the Ni/Fe ratio of each sample can be calculated by the following formula:

$$\frac{Ni}{Fe} = \frac{I_{Ni}(E_b)}{I_{Fe}(E_b)} \frac{T(E_{Ni})}{T(E_{Fe})} \frac{\sigma_{Fe}}{\sigma_{Ni}} \qquad (eq. 1)$$

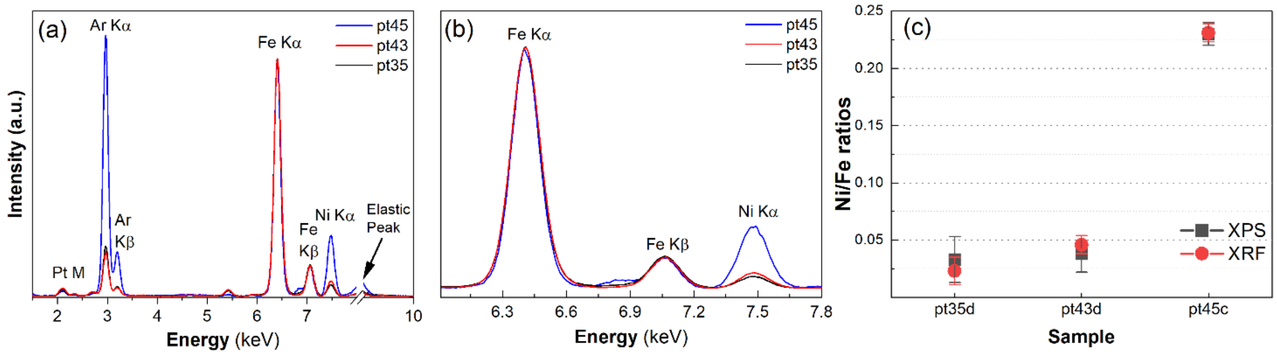


**Figure 2S.** (a) full XRF spectra of two selected samples (elastic peak was hidden to improve visualization); (b) Fe and Ni K emission lines; (c) Ni/Fe ratios obtained via XPS and XRF.

T($E_{Ni}$) and T($E_{Fe}$) are the transmittances in the optical path for the energy of the emission line of nichel (7.48 keV) and iron (6.4 keV) while σ is the *total X-ray fluorescence cross-section*, defined as the product of the *photoelectric cross section* of the shell at the given beam energy, the fluorescence yield and the fractional emission rate [4]. The values of the XRF cross sections for the Ni and Fe K edges at 8.6 keV were extrapolated from tabulated results [5]. As shown in Figure 2S-c, the results obtained via XRF are all within the experimental error of the XPS results (see tab. 1S).

| Sample | Thickness [nm] | Ni/Fe (XPS) | Ni/Fe (XRF) | Name |
|---|---|---|---|---|
| **Pt35** | 4 ± 0.5 | 0.033 ± 0.015 | 0.023 ± 0.011 | $Ni_{0.07}Fe_{2.62}O_4$ |
| **Pt43** | 4 ± 0.5 | 0.038 ± 0.015 | 0.046 ± 0.005 | $Ni_{0.1}Fe_{2.6}O_4$ |
| **Pt45** | 4 ± 0.5 | 0.23 ± 0.01 | 0.231 ± 0.009 | $Ni_{0.53}Fe_{2.3}O_4$ |

**Table 1S.** Ni/Fe ratios estimated via XPS and XRF analysis. In red, the corresponding name used in the main text.

## S2. OPERANDO XRF

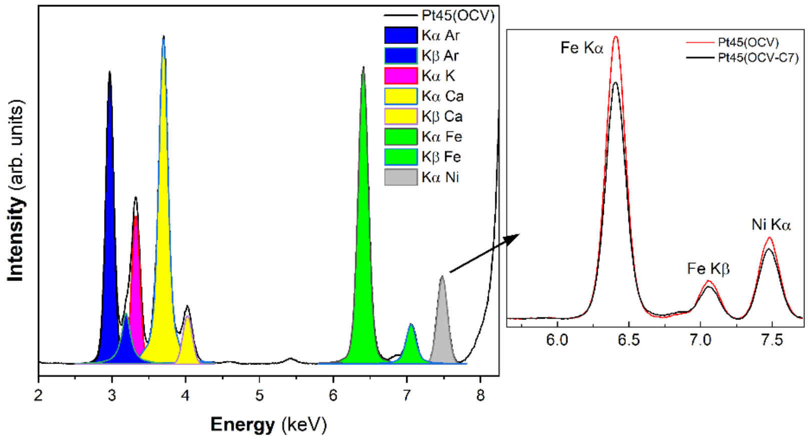


**Figure 3S**. XRF of sample pt45 after the electrolyte insertion (OCV). The elastic peak at 8.6 keV has been excluded to improve visualization. On the right, the emission lines of Ni and Fe after 7 cycles in the OCV-2.09 V window (OCV-C7) are confronted.

To check for the possible dissolution of Ni and Fe particles into the electrolyte, the Kα intensities of Fe and Ni have been acquired from sample pt45 just after inserting the electrolyte and after performing 7 cycles in the potential window 1.15 to 2.09 V Vs RHE with a scan rate of 20 mV/s. After normalizing the spectra for the intensity of the respective elastic peak, the relative intensity of the Fe and Ni emission lines are directly correlated to the number of Fe and Ni atoms in the sample. As shown by the spectra in figure 3S, the presence of the 0.1 M KOH is highlighted by the presence of the K lines of potassium and calcium. In the inset on the right, the spectra have been normalized to the respective incident beam intensity: it is shown that both Fe and Ni intensity is moderately lower after 7 cycles (-16% Fe and -14% Ni). However, considering that there is no clear change in the Ni/Fe ratios, this hindering could be also attributed to a slightly higher liquid layer thickness in the second measurement (C7).

## S3. Electrochemical Analysis

The electrochemical reliability of the cell was tested cycling 10 nm thin Ni film deposited via sputtering on flat Ti substrate (Goodfellow, 0.125 mm, 99.99%). The ohmic drop was measured via the current interrupted method integrated in the EC-Lab software. Figure 4S show how the resistance increase as the liquid layer thickness above the sample is reduced, resulting in a variation of the ohmic drop of the system. By applying 99% iR correction, the shift of the applied potential is completely removed. Slightly broader features at a fast scan rate can still be observed when the liquid layer thickness is minimized (Figure 4Sb) suggesting possible charge transport limitation.

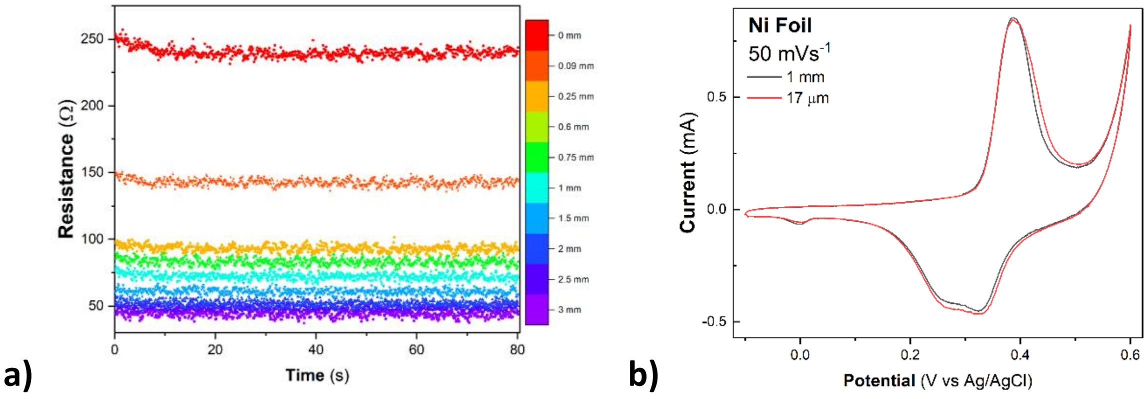


**Figure 4S.** (a) Resistance Vs time measured in current interrupted mode at different Z position. (b) iR corrected cyclic voltammetry for two different liquid layer thickness.

As discussed by Jan Myland et al [10], the uncompensated resistance of a three-electrode electrochemical cell can be schematized as the electrolyte resistance between working and reference electrode. In our experiment, we measured the resistance of the cell using current interrupt method integrated in the EC-lab software. The sample connected at the working electrode was a 0.125 mm thick, 1 cm diameter Ti substrate, with 10 nm Ni film deposited via sputtering. Each measure was carried out while flowing at 1.7 ml/min a solution of 1 M KOH, averaging the results for 80 s applying 500 μA (faradaic regime) and confronted with the values obtained at 50 μA (non-faradaic regime). The measure was repeated at different Z positions, with Z being the distance between the sample holder surface below the sample (WE) and the spacer.

At low frequency, the resistance from the WE and the reference electrode can be schematized like 3 resistors in series:

1. the volume of electrolyte above the sample surface ($R_s$)
2. the hollow cylinder between the counter electrode and the working electrode ($R_C$)
3. The electrolyte volume in the tube connecting the CE compartment to the reference electrode ($R_{ref}$).

Hence, similarly to the procedure presented in ref [10] we can calculate the total resistance as:

$$R(k,z) = R_s + R_c + R_{ref} = \frac{z - t_s}{A_s k} + \frac{\Delta R}{2\pi z k} \cdot \int_{R_{WE}}^{R_{CE}} \frac{dr}{r} + \frac{1}{k}\frac{d_r}{A_t}$$

With $A_s$ and $A_t$ area of the sample and tube respectively, ΔR the difference of radius between the working and counter electrode and k conductivity of the electrolyte, which can be calculated from the equation proposed by ref [11] from the molarity (M) and temperature of the solution(T = 296 K):

$$k = -2.041 * M + B * M^2 + C * M * T + D * \frac{M}{T} + E * M^3 + F * (M^2 * T^2)$$

Which gives in our case, for M = 1 mol/l and T = 296 K, gives a conductivity of 0.021 S/mm. The factor $z$-$t_s$ in the first term is due to the fact that we have to remove the volume occupied by the sample, of thickness $t_s$. However, if the first

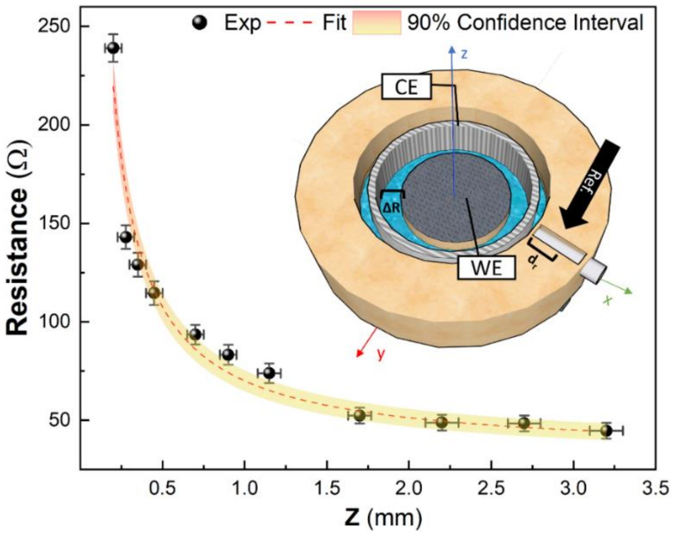


**Figure 5S.** Fit of the ohmic resistance of the cell as a function of z (working electrode/window distance) with flowing solution of 1 M KOH. In the inset, a sketch of the cell body (electrolyte in azure).

term is negligible for low z and large sample areas, the lower resistivity of the metallic sample should favor the electrons flow toward the sides of the sample at higher z values. The absence of an increase in resistance above 2 mm observed in our experiment confirm this hypothesis, an hence the first term can be neglected. Inserting the geometrical parameters of our cell, we find:

$$R(k,z)=\frac{0.82\ [mm]}{k}\frac{1}{z}+\frac{0.71}{k}$$

The second term, due to the reference electrode distance, does not depend significantly from z, and for big z (above 3 mm) gives the minimal resistance of ~30 Ω observed. Using this equation, the experimental data have been fitted (see figure 11S) to estimate the value of k. Our results confirm the $z^{-1}$ dependency of the resistance with z. The fitted value of k was 0.022 ±0.001 S/mm, in good agreement with the theoretical value.

To test the reliability of this model, we performed cyclic voltammetry on a Nichel foil and on the Ni film on Ti previously described. As shown in figure 6Sa, we find a clear $Ni^{2+}/Ni^{3+}$ oxidation peak between 380 and 400 mV vs Ag/AgCl, and the relative cathodic peak around 320 mV. Converting to the RHE electrode, we obtain at 100 $mVs^{-1}$ a anodic peak at 1.43 V and a cathodic peak at 1.35 V.

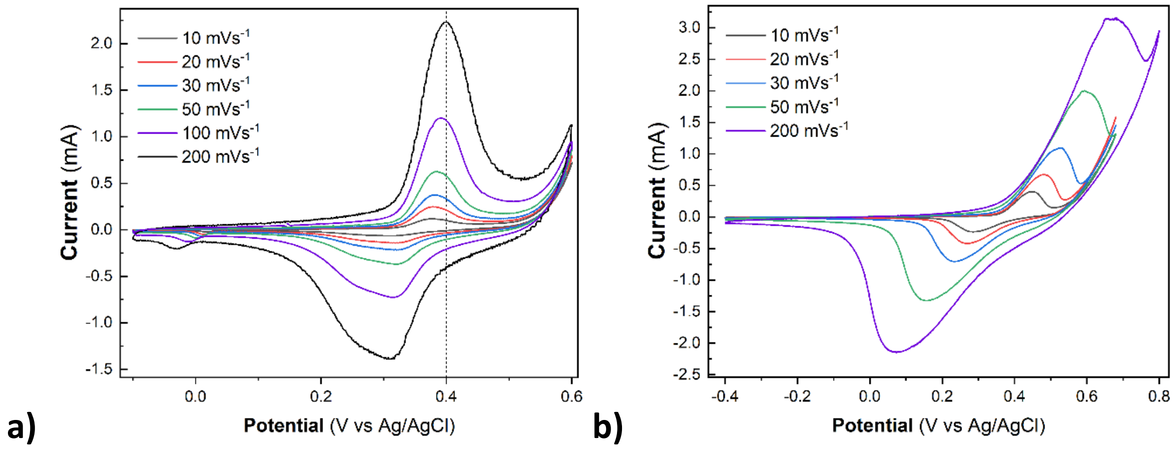


**Figure 6S.** Cyclic voltammetry at different scan rates on 10 nm Ni film (a) and 0.1 mm thick Ni foil (b) in 1 M KOH.

These result are in excellent agreement with other works on Ni/NiO films [13,14] and suggest the following reaction:

$$NiO+\ OH^{-}\ \leftrightarrow NiOOH+\ e^{-}$$

In Figure 6Sb, the much more evident shift of both peaks position suggest a much less reversible oxidation process on the pure Ni foil.

## S4. XAS

On the *as prepared* samples, we observe an increase of the Fe K pre-edge intensity as a function of the Ni content of the film (see Fig. 7S). A similar effect was observed by inserting $Ti^{4+}$ ions into the vacant maghemite octahedral sites, that resulted in the increase of the structural order of the material [7]. As shown also by F. De Groot et al. [8], the intensity of the $Fe_2O_3$ peak at 7114 eV is dominated by the $Fe^{3+}$ ions in tetrahedral sites. If the Ni dopant where to replace the tetrahedrally coordinated Fe ions, the pre-edge feature should almost be absent, like in the case of hematite.

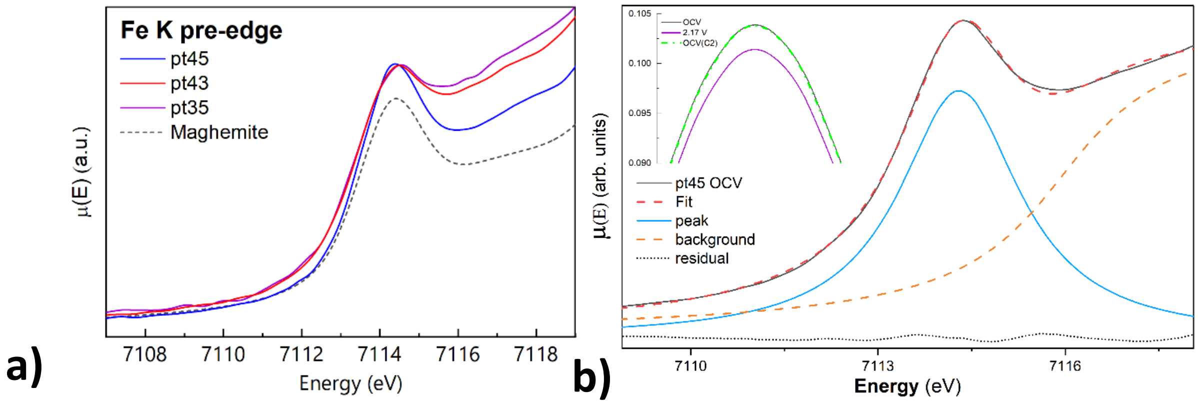


**Figure 7S.** a) Fe Pre-edge region of the XAS spectra. Samples are confronted to a spectrum acquired from a reference maghemite sample in transmission mode; b) fit of the Fe-K pre-edge.

Figure 8S show the linear combination fits performed on the XANES data acquired at the Ni K-edge. The fit has been carried out combining the spectra of pristine $NiFe_2O_4$ published in ref [9] and the spectra of the sample with lower Ni content (pt35). The increase of the white line intensity and a sharpening of the pre-edge region as the Ni content increase correlates with the gradual re-ordering of the sample towards $NiFe_2O_4$.

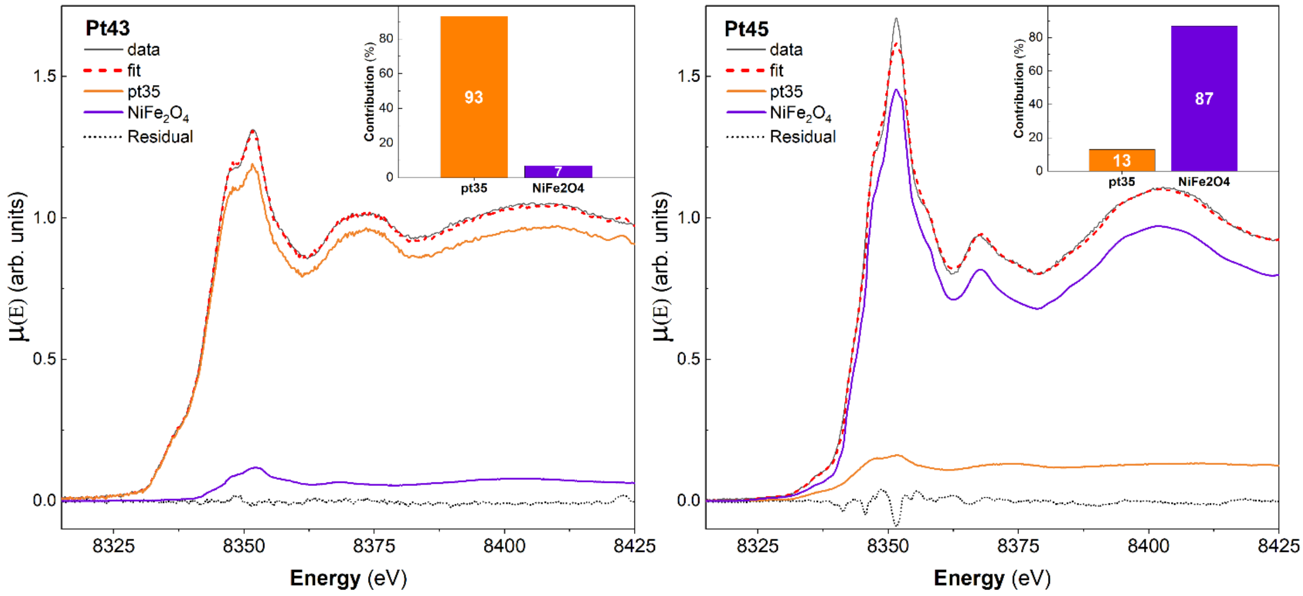


**Figure 8S.** Linear Combination fits of the XANES data at the Ni K-edge. In the insets, the bar graphs resume the results.

*Operando* measurements were carried out on pt35 to find the optimal parameters for the measurement. Sample pt35 was cycled in a wide potential range (-1 to +1.09 V vs Ag/AgCl). As shown in figure 9S, at oxidating potentials we observe

a small increase of the white line intensity on both Fe and Ni K edges, while the partial reduction from $Fe^{3+}$ to $Fe^{2+}$ at -1 V is confirmed by the negative shift of the spectra.

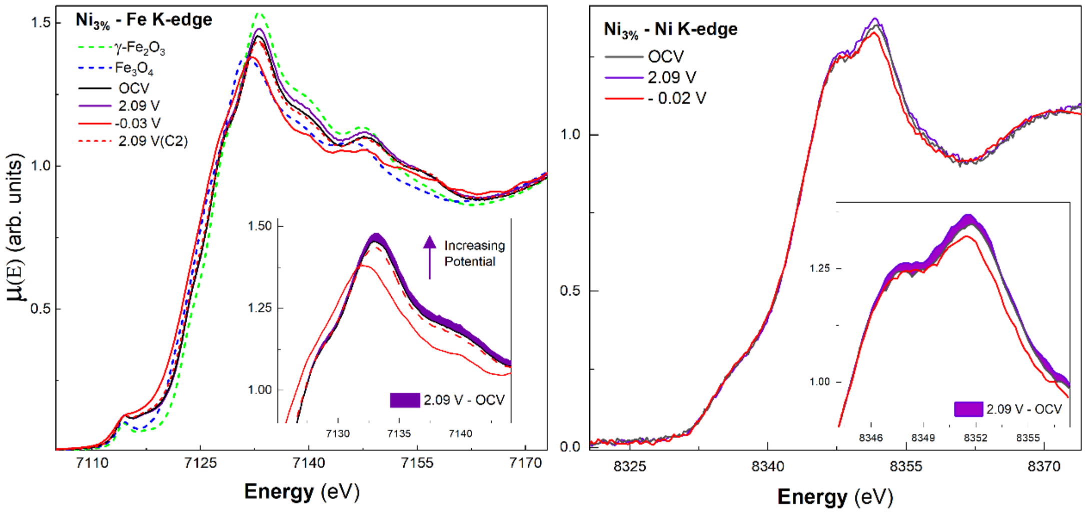


**Figure 9S.** Fe and Ni K-edges XANES vs applied potentials on sample pt35. In the insets, the purple area highlights the increase of the white line.

To confirm that the modulation of the white line discussed in the text was reproducible after several cycles, after 7 cycles (as in section S2) we repeated the measurement at the Fe and Ni K edges on sample pt45. The same trend is found again. Results are shown in figure 10S.

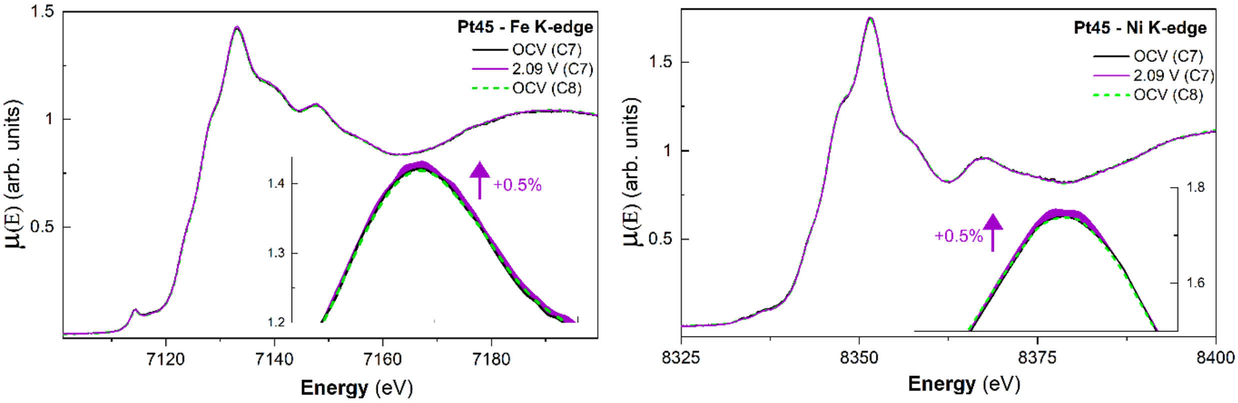


**Figure 10S.** Fe and Ni K-edges XANES for three charging state after 7 cycles: open circuit potential, 2.09 V and again back to OCV (C8, dashed lines). The white line changes are highlighted in the insets, together with the % increase of the intensity between 2.09 V and OCV (C7).

# S5. EXAFS

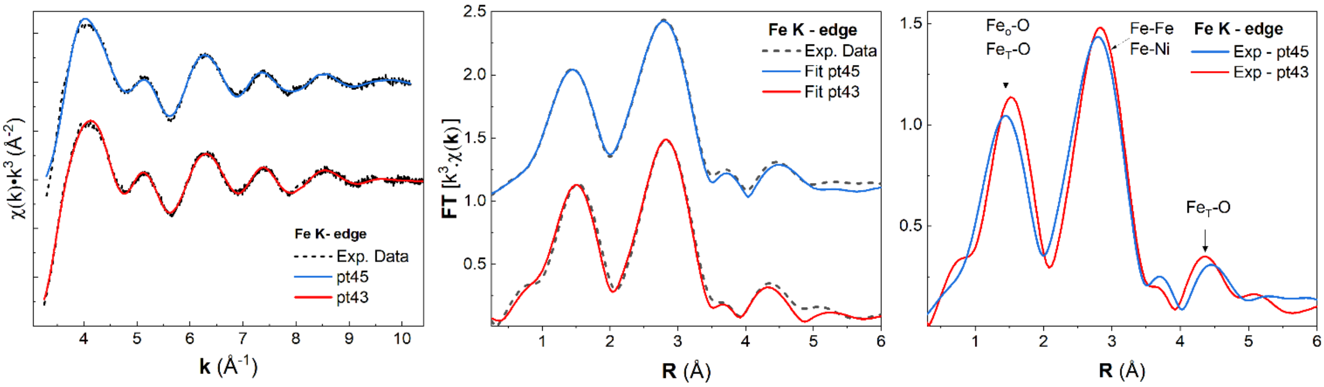

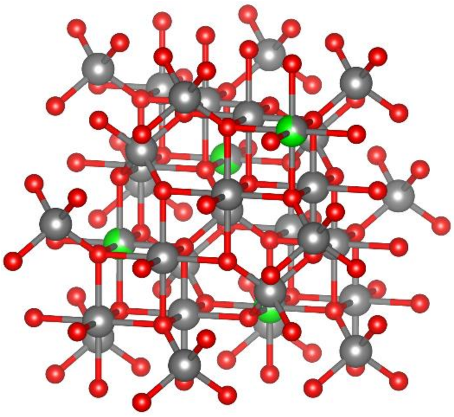

**Figure 11S.** The $k^3$-weighted EXAFS spectra at the Fe K-edge (left) and corresponding Fourier transform (center) relative to samples with 0.04 (in red) and 0.23 (blue) Ni/Fe ratios. On the right, the FT of the experimental data are superimposed to highlight the differences. Below, maghemite with Ni atoms in octahedral sites: in figure, the Fe atoms are in grey, oxygen is in red, while the green and grey positions are occupied by Ni (occupancy 0.667) or Fe (occupancy 0.333).

Fe K-edge EXAFS data of the samples at OCV where fitted using the GNXAS package. The initial structure employed was maghemite with cubic symmetry, with the octahedral Fe vacancies replaced by Ni atoms (see figure 11S). The fit was performed using XAS two-body signals, relative to the two-body distribution functions associated with different Fe-O, Fe-Ni and Fe-Fe bonds within the first two coordination shells. The signals from two non-equivalent photoabsorbers (Fe in tetrahedral and octahedral sites) were simulated from the proposed unit cell (space group cubic $P4_13_2$). The coordination numbers were fixed to the theoretical values while, following the results of ref [12], the first three shells of both photoabsorbers were included, varying debye-waller factors and distances in small ranges close to the expected values. Founded the optimal values, $Fe_T$-Ni and $Fe_O$-Ni first shells were included as well, fitting the Ni coordination number. The best-fit results are presented in table 2S.

| Fe K-edge | Theo. | (*) | Pt43 | | | Pt45 | | |
|---|---|---|---|---|---|---|---|---|
| **Shell** | **CN** | **R(Å)** | **CN** | **R(Å)** | $\sigma^2$(Å) $\cdot 10^2$ | **CN** | **R(Å)** | $\sigma^2$(Å) $\cdot 10^2$ |
| **$Fe_O$-O** | 6 | 2.08 | 6 | $2.02 \pm 0.03$ | $0.9 \pm 0.3$ | 6 | $2.00 \pm 0.02$ | $0.22 \pm 0.08$ |
| **$Fe_T$-O** | 4 | 1.80 | 4 | $1.91 \pm 0.03$ | $0.3 \pm 0.1$ | 4 | $1.85 \pm 0.02$ | $0.13 \pm 0.05$ |
| **$Fe_O$-$Fe_O$** | 5 | 2.95 | 5 | $3.05 \pm 0.02$ | $0.21 \pm 0.08$ | 5 | $3.03 \pm 0.03$ | $0.27 \pm 0.08$ |
| **$Fe_O$-Ni** | 1 | 2.95 | $1 \pm 0.1$ | $3.02 \pm 0.03$ | $0.6 \pm 0.1$ | $1.4 \pm 0.2$ | $2.97 \pm 0.03$ | $0.9 \pm 0.2$ |
| **$Fe_T$-Ni** | 3 | 3.45 | $3 \pm 0.3$ | $3.54 \pm 0.04$ | $0.4 \pm 0.1$ | $4.2 \pm 0.6$ | $3.57 \pm 0.05$ | $0.3 \pm 0.1$ |
| **$Fe_T$-$Fe_O$** | 10 | 3.45 | 10 | $3.51 \pm 0.05$ | $1.9 \pm 0.3$ | 9 | $3.47 \pm 0.03$ | $1.1 \pm 0.1$ |
| **$Fe_O$-$Fe_T$** | 6 | 3.45 | 6 | | | 6 | | |
| **$Fe_T$-$Fe_T$** | 4 | 3.61 | 4 | $3.79 \pm 0.09$ | $0.6 \pm 0.1$ | 4 | $3.77 \pm 0.04$ | $0.2 \pm 0.2$ |
| ***$Fe_T$-$Fe_O$** | 3 | 5.41 | 3 | $4.8 \pm 0.1$ | $1.3 \pm 0.2$ | 3 | $5.2 \pm 0.2$ | $0.90 \pm 0.1$ |
| ***$Fe_T$-Ni** | 1 | 5.41 | $1 \pm 0.1$ | | | $1.4 \pm 0.2$ | | |

**Table 2S.** Best-fit values of the EXAFS spectra at the Fe K-edge. $Fe_T$ indicate the photoabsorber in the tetrahedral site, while $Fe_O$ the one in octahedral sites. Theoretical values of CN and R for the proposed structure are given in the 2° and 3° columns. Debye-Waller factors ($\sigma^2$) have been multiplied by a $10^2$ factor to improve visualization. The 7° and 10° rows are left blank because those two body signals were fitted with the same parameters as the line above.

The fitted R values are in good agreement with the theoretical values of maghemite. The fitted $\sigma^2$ values are also in a similar range with respect to the results of ref [12], with the higher values within the first shell of sample pt43 that suggest a lower structural order respect to the Ni-rich sample.

As discussed in the main text no clear change is observed in the EXAFS signal in *operando* conditions (figure 12S).

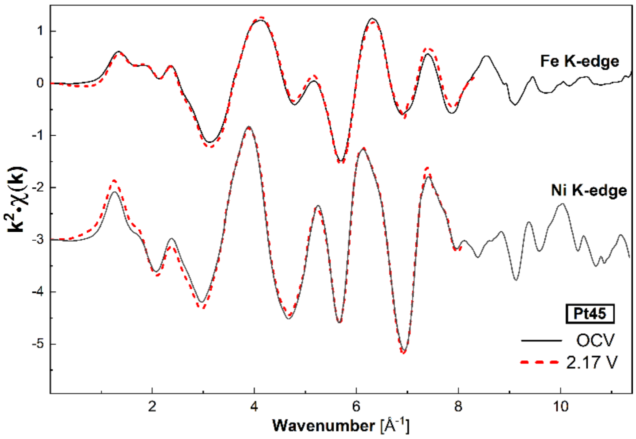


**Figure 12S.** EXAFS data at the Fe (top) and Ni (bottom) K-edges acquired in *operando* conditions at open circuit potential (black) and 2.09 V (dashed red) on $Ni_{23\%}Fe_2O_3$.

## S6. Electrolyte thickness

In a precedent experiment, the electrolyte thickness was estimated with the same procedure described in the text, acquiring the fluorescence spectra from an iridium sample, with incident beam energy of 11.6 keV (see figure 13S-a). Without using the Teflon mask (Figure 13S-b), the elasticity of the Kapton window result in a non-linear behavior as a function of the substrate movement, as well as a final thickness significantly higher than the one shown in the text, due to the bumping of the window. In fact, after the sample is brought in contact with the spacer and pressed towards the window, the latter tend to follow the substrate while it is moved away from it. When the sample is moved ~1.5-2 mm away from the initial position, the spacer completely detach from the sample, the thickness of the liquid layer increase and, hence, the intensity of the fluorescence signal drastically decrease. The experimental error was approximated as the standard deviation of the measures. When the sample is in perfect contact with the spacer, the calculated value (64 ± 15 µm) agrees with the nominal thickness of the spacer employed (50.7 µm).

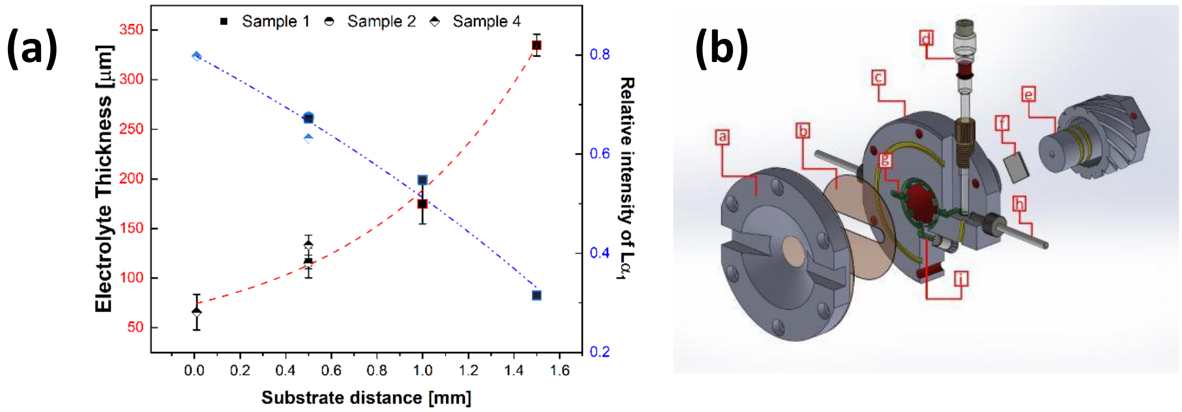


**Figure 13S.** (a) Calculated value of the electrolyte layer thickness at different distances from the Kapton window without the Teflon mask. In blue, the relative intensity (respect to the signal measured without liquid) of the $L\alpha_1$ emission line of iridium. In red the calculated thickness. (b) Exploded view of the electrochemical cell without the mask: a) cell window and mask assembled, b) spacer, c) cell body, d) reference electrode, e) sample holder column, f) sample, g)electrolyte inlet and outlet (h), i) couter electrode wire compartment.

Using the Teflon mask, a regular exponential decay of the transmittance as a function of the substrate position was observed (Fig 14S), due to a linear dependance of the electrolyte thickness to the substrate movement, with a minimal liquid layer thickness much lower than the spacer thickness.

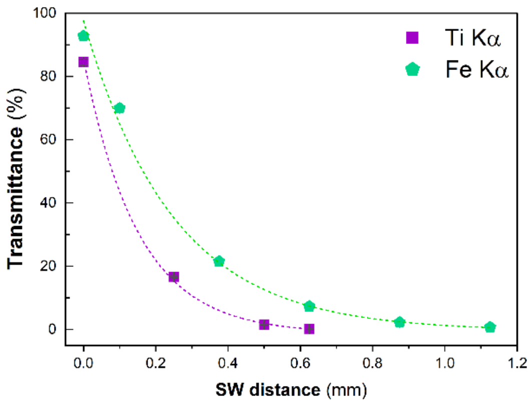


**Figure 14S.** Intensity ratio of the Kα line with and without the liquid layer, as a function of the sample-window distance. The exponential trends have been calculated from the measurements on two different samples, titanium (purple) and iron (green).

## REFERENCES.

[1] G. Liu et al., "*Uniformly mesoporous NiO/NiFe$_2$O$_4$* biphasic nanorods as efficient oxygen evolving catalyst for water splitting", Int. Jour. Of Hydrogen energy 41 (2016), 17976-17986.

[2] M. Hua et al., "*Hexamethylenetetramine-assisted hydrothermal synthesis of octahedral nickel ferrite oxide nanocrystallines with excellent supercapacitive performance*", J. Mater. Sci. Energy Materials

[3] M. McBriarty, "*Atomic Scale Structure-Chemistry relationships at oxide catalysts surfaces and interfaces"* (2014), in Materials Science and Engineering, Northwestern University.

[4] J.A. Klung, "*Synchrotron X-ray studies of epitaxial ferroelectric thin films and nanostructures"* (2010) in Physics and Atronomy, Northwestern University.

[5] T. Schoonjans et al., "*The xraylib library for X-ray-matter interactions. Recent developments"* (2011), Spectrochimica Acta Part B, 776-784.

[7] J. Chen et al., "*Simultaneously enhancing stability and activity of maghemite via site-specific Ti(iv) doping for no emission control*", ChemCatChem 10, 4683 (2018).

[8] F. de Groot et al., "*The 1s x-ray absorption pre-edge structures in transition metal oxides*", Journal of Physics: Condensed Matter 21, 104207 (2009).

[9] Q. Yue et al., "*Defect engineering of mesoporous nickel ferrite and its application for highly enhanced water oxidation catalysis"*, Journal of Catalysis 358 (2018) 1-7.

[10] J. C. Myland and K. B. Oldham., "*Uncompensated resistance. 1. the effect of cell geometry*", Analytical Chemistry 72, 3972 (2000).

[11] R.J. Gilliam et al., "*A review of specific conductivities of potassium hydroxide solutions for various concentrations and temperatures.*", International Journal of Hydrogen energy 32, (2007) 359-364.

[12] M. Coduri et al., "*Local structure and magnetism of Fe$_2$O$_3$ maghemite nanocrystals: The role of crystal dimension .*", Nanomaterials 10 (2020).

[13] M.S.A. Akbari et al., "*Oxygen-evolution reaction by nichel/nickel oxide interface in the presence of ferrate(VI).*", Scientific Reports 10 (2020) 8757.

[14] B.T. Sone et al., "Physical & Electrochemical Properties if Green Synthesized Bunsenite NiO Nanoparticles via callistemon Viminalis' Extracts.", International Journal of Electrochemical Science 11 (2016) 8204-8220.

[15] N. Fairley et al., "Systematic and Collaborative Approach to Problem Solving using X-ray Photoelectron Spectroscopy.", Applied surface science advances 5 (2021),100112.
